# Supplementary material for: Neural Scene Representation for Locomotion on Structured Terrain
Source: arXiv:2206.08077 source file (2022-06-16)
Supplement: Supplementary file 1 [file 6_appendix.tex]

\appendix
\subsection{Architecture and Training}
\label{app:training}
The sequence of down-sampling convolutions produce features maps of dimension 8, 16, 32, 64, 128, in that order. The normal and strided convolutions in the encoder have a kernel size of $[3,3,3,2]$ and $[2,2,2,2]$, respectively. The normal and strided convolutions in the decoder have a kernel size of $[3,3,3,1]$ and $[2,2,2,1]$, respectively. After every convolution we use batch normalization and an ELU activation function, expect for the output, which has a Sigmoid activation.

We train our model using the ADAM optimizer with a mini batch size of 32 for a total of 40 epochs. The initial learning rate of $0.01$ is decayed exponentially every epoch up to a value of $0.0001$.

The validation data is collected on trajectories in newly randomized environments. 

\subsection{Hardware Experiments}
\label{app:setup}
For each experiment, we use the following amount of data:
\begin{itemize}
    \item \emph{Stairs A} consists of 264 time steps for a total of 1'518'111 points in the ground truth map
    \item \emph{Stairs B} consists of 176 time steps with 1'116'540 points in the ground truth map
    \item \emph{Boxes}
\end{itemize}

\subsection{Pre-drift Performance}
\label{app:pre_drift}
\begin{table}[h]
    \centering
    \caption{Comparison of the different approaches on the \emph{Stairs A} data set up to the drift.}
    \begin{tabular}{c | c c c c c}
        \hline
        { } & {Method} & \makecell{Pr. [$\%$]} & \makecell{Re. [$\%$]} & \makecell{F1 [$\%$] } & \makecell{MAE [$\SI{}{\centi\meter}$] } \\
        \hline
        \multirow{4}*{\rotatebox[origin=c]{90}{\textbf{Stairs A}}} & {Measurement} & $88.4$ & $50.5$ & $63.9$ & $0.6$ \\
                                       & E.M. \cite{Fankhauser2018ProbabilisticTerrainMapping} &  $81.1$ & $84.9$ & $82.9$ & $1.2$ \\
                                       & {Voxblox \cite{oleynikova2017voxblox}} & $78.9$ & $69.0$ & $72.5$ & $1.5$ \\
                                       & {Ours} & $\mathbf{87.6}$ & $\mathbf{89.4}$ & $\mathbf{88.5}$ & $\mathbf{0.9}$ \\
        \hline
    \end{tabular}
    \label{tab:comparison_drift}

\end{table}

\begin{table}[h]
    \centering
    \caption{Comparison of the different approaches on the \emph{Stairs A} data set up to the drift.}
    \begin{tabular}{c | c c c c c}
        \hline
        { } & {Method} & \makecell{Pr. [$\%$]} & \makecell{Re. [$\%$]} & \makecell{F1 [$\%$] } & \makecell{MAE [$\SI{}{\centi\meter}$] } \\
        \hline
        \multirow{4}*{\rotatebox[origin=c]{90}{\textbf{Stairs A}}} & {Measurement} & $88.4$ & $50.5$ & $63.9$ & $0.6$ \\
                                       & E.M. \cite{Fankhauser2018ProbabilisticTerrainMapping} &  $79.9$ & $83.8$ & $81.7$ & $1.3$ \\
                                       & {Voxblox \cite{oleynikova2017voxblox}} & $78.3$ & $69.0$ & $72.2$ & $1.5$ \\
                                       & {Ours} & $\mathbf{87.6}$ & $\mathbf{89.4}$ & $\mathbf{88.5}$ & $\mathbf{0.9}$ \\
        \hline
    \end{tabular}
    \label{tab:comparison_drift}

\end{table}

\subsection{ICP Registration}
\label{app:icp}
To carry out the ICP registration between the measurements and the ground truth map, we additionally use the point cloud from a Velodyne scanner on the robot. The Velodyne data has a longer range and  constrains the ICP optimization further by including more elements such as walls, see Fig.~\ref{fig:icp}. Following the alignment, the point cloud around the robot in the BLK2GO map is taken as ground truth. We use Open3D~\cite{Zhou2018} for registration.
\begin{figure}[h]
    \centering
    \begin{subfigure}[b]{\columnwidth}
        \centering
        \includegraphics[width=\columnwidth]{images/icp_pre_alignment.png}
     \end{subfigure}
    \begin{subfigure}[b]{\columnwidth}
        \centering
        \includegraphics[width=\columnwidth]{images/icp_aligned.png}
    \end{subfigure}
    \caption{Example ICP alignment result. The measurements (yellow) are obtained by combining the measurements from the 4 Realsense cameras and the Velodyne LiDAR, and the ground truth (blue) using the BLK2GO LiDAR scanner. The initial alignment (top) has an offset of a couple of meters and around 180 degrees, while the ICP registration (bottom) results in a tight fit.}
    \label{fig:icp}
\end{figure}
